# Supplementary material for: RevPHiSeg: A Memory-Efficient Neural Network for Uncertainty Quantification in Medical Image Segmentation
Source: arXiv:2008.06999 source file (2020-08-18)
Supplement: Supplementary file 1 [file appendix.tex]

\section{Appendix}
\subsection{Memory consumption for different batch sizes}
In Fig.\ref{fig:memory_batch} one can see the memory consumption for different batch sizes. It is interesting to note that the memory footprint of the reversible architecture does not grow with the same rate as the original architecture.
\begin{figure}[h]
    \centering
    \begin{tikzpicture}
    \begin{axis}
        [xlabel=Batch size,
        ylabel=Memory consumption in GB,
        grid=major,
        legend pos=south east]
        \addplot table [y=mem, x=batch]{data/memory.dat};
        \addlegendentry{PHiSeg}
        \addplot table [y=mem_rev, x=batch]{data/memory.dat};
        \addlegendentry{RevPHiSeg}
        \end{axis}
    \end{tikzpicture}
    \caption{Memory consumption of PHiSeg and the reversible PHiSeg on the LIDC dataset for different batch sizes}
    \label{fig:memory_batch}
\end{figure}{}
